# Supplementary material for: ZigZagkv: Dynamic KV Cache Compression for Long-context Modeling based on Layer Uncertainty
Source: arXiv:2412.09036 source file (2024-12-12)
Supplement: Supplementary file 1 [file appendix.tex]

\onecolumn
\newpage
\appendix
\section{Appendix}
\subsection{Detailed Needle Results}
\label{detail_needle}

\subsection{Detailed LongBench Results}
\input{Tables/longbench_llama3_1}
